# Supplementary material for: Rzk: a Proof Assistant for Synthetic $\infty$-Categories
Source: arXiv:2607.12207 source file (2026-07-13)
Supplement: Supplementary file 1 [file appendix-eta-subsumption.tex]

\section{Pointwise Subsumption: a Possible Extension of \dRzk{}}
\label{app:eta-subsumption}

In \cref{sec:subtyping} we saw one silent passage of \RSTT{} that subtyping cannot capture. In
the forward direction of the composition law for cofibrations (\cref{ex:cofibration-composition}),
a section $h : \ty{\prod}_{\pt{t} : \{\cube{I} \mid \tp{\chi}\}} \ty{X}(\pt{t})\,[\, \tp{\phi}(\pt{t}) \mapsto a(\pt{t}) \,]$
is re-used at the type
$\ty{\prod}_{\pt{t} : \{\cube{I} \mid \tp{\chi}\}} \ty{X}(\pt{t})\,[\, \tp{\psi}(\pt{t}) \mapsto h(\pt{t}) \,]$,
whose boundary pins the values of $h$ itself. The passage is sound for $h$ but not for an
arbitrary inhabitant of $h$'s type, so no subtyping rule can license it, and \dRzk{} accepts only
the $\eta$-expanded witness $\lambda \pt{t}.\, h(\pt{t})$. This appendix records the extension
that would accept the $\eta$-reduced witness as well, shows that it is a genuinely new rule, and
lists what adopting it would touch in the metatheory and in the implementation. Finally, we
record a dual subtyping rule, which collapses a restriction in the region where its tope holds
(\cref{app:eta-sub-dual}). We adopt neither extension in this paper.

\subsection{The Rules}
\label{app:eta-sub-rules}

The extension is a term-level companion to \textsc{T-Sub}, \emph{pointwise subsumption}, in a
shape form and an ordinary form:
\begin{prooftree}
  \AxiomC{$\cube{\Xi} \mid \tp{\Phi} \mid \ty{\Gamma} \vdash f : \ty{\prod}_{\pt{t} : \{\cube{I} \mid \tp{\psi}\}} \ty{B}(\pt{t})$}
  \AxiomC{$\cube{\Xi}, \pt{t} : \cube{I} \mid \tp{\Phi}, \tp{\psi}(\pt{t}) \mid \ty{\Gamma} \vdash f(\pt{t}) : \ty{D}(\pt{t})$}
  \RightLabel{\textsc{T-Sub-$\eta$-shape}}
  \BinaryInfC{$\cube{\Xi} \mid \tp{\Phi} \mid \ty{\Gamma} \vdash f : \ty{\prod}_{\pt{t} : \{\cube{I} \mid \tp{\psi}\}} \ty{D}(\pt{t})$}
\end{prooftree}
\begin{prooftree}
  \AxiomC{$\cube{\Xi} \mid \tp{\Phi} \mid \ty{\Gamma} \vdash f : \ty{\prod}_{y : \ty{A}} \ty{B}(y)$}
  \AxiomC{$\cube{\Xi} \mid \tp{\Phi} \mid \ty{\Gamma}, y : \ty{A} \vdash f(y) : \ty{D}(y)$}
  \RightLabel{\textsc{T-Sub-$\eta$}}
  \BinaryInfC{$\cube{\Xi} \mid \tp{\Phi} \mid \ty{\Gamma} \vdash f : \ty{\prod}_{y : \ty{A}} \ty{D}(y)$}
\end{prooftree}
Each rule is the corresponding $\eta$-rule read as a typing principle:
$\lambda \pt{t}.\, f(\pt{t})$ inhabits the conclusion by \textsc{$\Pi$-intro-shape}, and
$f \equiv \lambda \pt{t}.\, f(\pt{t})$ by \textsc{$\Pi$-$\eta$-shape}, so the rule lets the
typing of $f$ follow that of its $\eta$-expansion without changing the term. In particular, both
rules are sound in any model validating the $\eta$-rules, since $f$ and its $\eta$-expansion have
the same interpretation. Like \textsc{T-Sub}, both rules are silent and coercion-free. There is
deliberately no $\ty{\Sigma}$ variant, matching the implementation below and the minimal-spine
choice of \cref{def:ext-style}.

With the rules, the forward map of \cref{ex:cofibration-composition} checks in its
$\eta$-reduced form $\lambda h.\, (h, h)$: by \textsc{T-Sub-$\eta$-shape} it suffices that, under
$\pt{t} : \tp{\chi}$, the application $h(\pt{t})$ inhabits
$\ty{X}(\pt{t})\,[\, \tp{\psi}(\pt{t}) \mapsto h(\pt{t}) \,]$, which follows by
\textsc{S-Restr$'$} and \textsc{Restr-intro}, the boundary premise holding by reflexivity.

\subsection{The Rules are not Derivable}
\label{app:eta-sub-underivable}

The rules are not derivable from the $\eta$-rules and \textsc{T-Sub}; indeed, they are not even
admissible in \dRzk{}. Judgemental $\eta$ identifies $f$ with $\lambda \pt{t}.\, f(\pt{t})$ as
terms, but no rule of \dRzk{} transfers a typing along an equality of terms: conversion,
\textsc{T-Sub} with \textsc{S-Conv}, rewrites the type of a judgement, not its subject. For the
types displayed above, $\lambda \pt{t}.\, h(\pt{t})$ inhabits the second while the variable $h$
does not: by the generation property of \cref{app:coh-placement}, a typing of $h$ can only
combine its context type with \textsc{T-Sub} and \textsc{Restr-intro} steps;
\textsc{Restr-intro} attaches a restriction only at the root, and the required \textsc{S-Restr}
premise fails, since $\tp{\psi}$ does not entail the strictly smaller $\tp{\phi}$. Thus the
rules assert precisely that typing is invariant under $\eta$-contraction of the subject, which
the $\eta$-equality alone does not provide.

Alternatively, both rules become derivable in the presence of a general \emph{subject
conversion} rule (from $t \equiv u$ and $u : \ty{B}$ conclude $t : \ty{B}$). We consider that
rule too strong: it makes typing invariant under all of $\beta\eta$ on subjects, well beyond
what the type checker performs, and it invalidates the generation property on which the
coherence proof of \cref{app:coherence} rests.

\subsection{What Adopting the Rules Would Touch}
\label{app:eta-sub-impact}

Adopting the rules leaves the statements of \cref{thm:faithfulness,thm:conservativity} unchanged,
but their proofs quantify over \dRzk{} derivations, so each inductive argument gains a case:
\begin{itemize}
  \item \emph{Silent steps} (\cref{app:coh-placement}). Exactly \emph{three} rules, rather than
    two, then conclude a typing without analysing the term. The generation property changes
    shape: a \textsc{T-Sub-$\eta$} step carries a sub-derivation whose subject is the
    application $f(\pt{t})$, so silent chains become nested rather than linear, and
    \cref{lem:chain-coherence} must be restated over the nested form. Its proof appears to
    extend: the $\sigma$-effect of a \textsc{T-Sub-$\eta$} step is
    $f \mapsto \lambda \pt{t}.\, c(f(\pt{t}))$, which is the uniform $\ty{\Pi}$-node form
    already handled by \cref{thm:coercion-coherence}.
  \item \emph{Back-translation} (\cref{def:backtranslation}). One new clause:
    $\sigma(\textsc{T-Sub-$\eta$}) = \lambda \pt{t}.\, \sigma(\text{premise})$. Under $\sigma$
    this is an extension-type (or $\ty{\Pi}$) introduction in \RSTT{}, whose side condition is
    exactly the boundary equation produced inside the premise, typically at
    \textsc{Restr-intro}; \cref{lem:backtranslation-sound} gains the corresponding case. Note
    that the back-translated term is the $\eta$-expansion that \RSTT{} writes anyway.
  \item \emph{The ext-style fragment} (\cref{def:ext-style-derivation}). The rules stay within
    it: the premise concludes a tail type, and no variable is bound at a non-ext-style type
    (the shape form binds a point; the ordinary form binds $y$ at the domain of $f$'s type).
  \item \emph{Conversion agreement} (\cref{sec:conservativity}). Unchanged: the rules add
    typings, not equalities.
\end{itemize}

In the implementation, the extension is a small change to the subtyping routine of
\cref{sec:checking-subtyping}. The routine already carries the term being checked and applies it
to the bound point when it descends into a $\ty{\Pi}$ codomain; the change is that a face
$[\, \tp{\phi} \mapsto s \,]$ of the expected type may be checked directly by comparing the carried
term with $s$ under $\tp{\phi}$, falling back to the coverage check corresponding to
\textsc{S-Restr}. We have prototyped this in a development version of the checker (after
v0.7.8, which this paper reports): the \sHoTT{} corpus is unaffected, and the $\eta$-reduced
forward map above checks. The \emph{fully} $\eta$-reduced proof of
\cref{ex:cofibration-composition} still does not: its round-trip witnesses need the equality of
two neutral terms of extension type, which \dRzk{} proves by \textsc{$\Pi$-$\eta$-shape},
congruence under the binder, and \textsc{Restr-comp}, but which the equality routine, comparing
neutral terms structurally, does not find. That incompleteness of algorithmic equality is
independent of the extension recorded here.

\subsection{A Dual Fragment: Collapsing a Satisfied Restriction}
\label{app:eta-sub-dual}

The reflexive-face passage is not the only silent step that amounts to transferring a typing
along a definitional equality. Consider the candidate subtyping rule
\begin{prooftree}
  \AxiomC{$\cube{\Xi} \mid \tp{\Phi} \mid \ty{\Gamma} \vdash \ty{A}\,[\, \tp{\phi} \mapsto a \,] \;\ty{\mathsf{type}}$}
  \AxiomC{$\cube{\Xi} \mid \tp{\Phi} \vdash \tp{\phi}$}
  \AxiomC{$\cube{\Xi} \mid \tp{\Phi} \mid \ty{\Gamma} \vdash a : \ty{B}$}
  \RightLabel{\textsc{S-Restr-Collapse}}
  \TrinaryInfC{$\cube{\Xi} \mid \tp{\Phi} \mid \ty{\Gamma} \vdash \ty{A}\,[\, \tp{\phi} \mapsto a \,] \subtype \ty{B}$}
\end{prooftree}
which collapses a restriction in the region where its tope holds: when $\tp{\Phi}$ entails
$\tp{\phi}$, every $x : \ty{A}\,[\, \tp{\phi} \mapsto a \,]$ is definitionally $a$
(\textsc{Restr-comp}), so the restricted type is a singleton at $a$ and embeds wherever $a$
lives. The rule is sound in any model, for an arbitrary $\ty{B}$, even one structurally
unrelated to $\ty{A}$.

The two extensions are the two halves of subject conversion, split by the boundary region.
\textsc{S-Restr-Collapse} transfers a typing along \textsc{Restr-comp}; its witness $a$ is stored in
the type, which is why it can be phrased as a pure subtyping at all, and it applies
\emph{inside} the region $\tp{\phi}$. \textsc{T-Sub-$\eta$} transfers a typing along
\textsc{$\Pi$-$\eta$-shape}; its witness is the $\eta$-expansion of the subject, which no type
stores, and it applies \emph{outside} the region, where the boundary is an obligation rather
than a computation. For the same reason, \textsc{S-Restr-Collapse} does not reach the reflexive-face
passage of \cref{app:eta-sub-rules}: there the comparison happens under $\pt{t} : \tp{\chi}$,
which entails neither $\tp{\phi}$ nor $\tp{\psi}$, and, being a pure subtyping rule, it is in
any case excluded by the quantification argument of \cref{app:eta-sub-underivable}.

Algorithmically, \textsc{S-Restr-Collapse} is the declarative shadow of the restriction computation
(\cref{sec:bidirectional}): the checker reduces $x$ to $a$ once $\tp{\phi}$ is entailed, so the
instances that arise in practice are absorbed by evaluation and, on expected faces, by the face
check described above. The residual strength of the rule, using $x$ at a type $\ty{B}$ not
convertible with $\ty{A}$, is beyond the checking algorithm, and we have not seen it needed in
the \sHoTT{} library. Its metatheoretic cost is also higher than that of \textsc{T-Sub-$\eta$}:
its $\sigma$-coercion is the constant map $x \mapsto \sigma a$ between types with unrelated
$\tp{\Phi}$-skeletons, which breaks the skeleton discipline (\cref{lem:skeleton}) that the
coherence proof of \cref{thm:coercion-coherence} rests on, rather than adding a uniform case to
it.
