# Supplementary material for: Rzk: a Proof Assistant for Synthetic $\infty$-Categories
Source: arXiv:2607.12207 source file (2026-07-13)
Supplement: Supplementary file 2 [file appendix-rec-path.tex]

\section{Tope Disjunction Elimination along Propositional Equality}
\label{app:rec-path}

The standard tope-disjunction eliminator $\mathsf{rec}_\lor(\psi \mapsto a_\psi, \phi \mapsto a_\phi)$
requires $a_\psi$ and $a_\phi$ to be \emph{definitionally} equal on $\psi \wedge \phi$. Sometimes
this is too strong: the two branches may agree only up to a path. Assuming extension-type
extensionality (\code{extext}, \cref{ex:segal-function-types}), one can define a weaker variant
\code{rec-path} that takes a witness of \emph{propositional} equality on the intersection and
produces a section over $\psi \vee \phi$. Riehl and Shulman use this trick in the proof of
multivariable covariance~\cite[Proposition~8.21]{RiehlShulman2017}, without factoring it out as a
standalone result. At the time of writing, it is being added to \sHoTT{} as
\code{rec-path}\footnote{See pull requests \#165 (\code{rec-path}) and \#163 (multivariable
covariance) of the \sHoTT{} library~\cite{shott}.} (module
\texttt{simplicial-hott/03-extension-types}):

\begin{minted}[frame=lines]{rzk}
#define rec-path uses (extext)
  ( a-in-ψ : (t : ψ) → A t)
  ( a-in-φ : (t : φ) → A t)
  ( e : (t : I | ψ t ∧ φ t) → a-in-ψ t = a-in-φ t)
  : ( t : I | ψ t ∨ φ t) → A t
  := ...
\end{minted}

The construction transports the restriction of \code{a-in-ψ} along the path supplied by the
extensionality axiom, so that it agrees definitionally with the restriction of \code{a-in-φ} on
$\psi \wedge \phi$, and then invokes the standard \code{recOR}. The trick recurs in synthetic $\infty$-category proofs
whenever two diagrams have to be glued along an intersection on which they agree only up to a
path, as in multivariable covariance~\cite[Proposition~8.21]{RiehlShulman2017}.

Here, the type-directed restriction computation of \cref{sec:bidirectional} drives the
coercion between an extension of a restriction and the underlying section; the tope solver
checks the $\psi \wedge \phi$ and $\psi \vee \phi$ side conditions
(\cref{sec:automated-tope-logic}); and definitional equality of the two branches is checked
branch-wise under each of $\psi$ and $\phi$ (\cref{sec:def-eq-topes}).
